# Supplementary material for: SkyByte: Architecting an Efficient Memory-Semantic CXL-based SSD with OS and Hardware Co-design
Source: arXiv:2501.10682 source file (2025-01-18)
Supplement: Supplementary file 1 [file appendix.tex]

% \appendix

% \subsection{Impact of Context Switching on SSD Access Latency}
% \label{appendix:eval_ctx_switch_ssd_latency}

% \begin{figure}[!tph]
%     \centering
%     \includegraphics[width=0.90\linewidth]{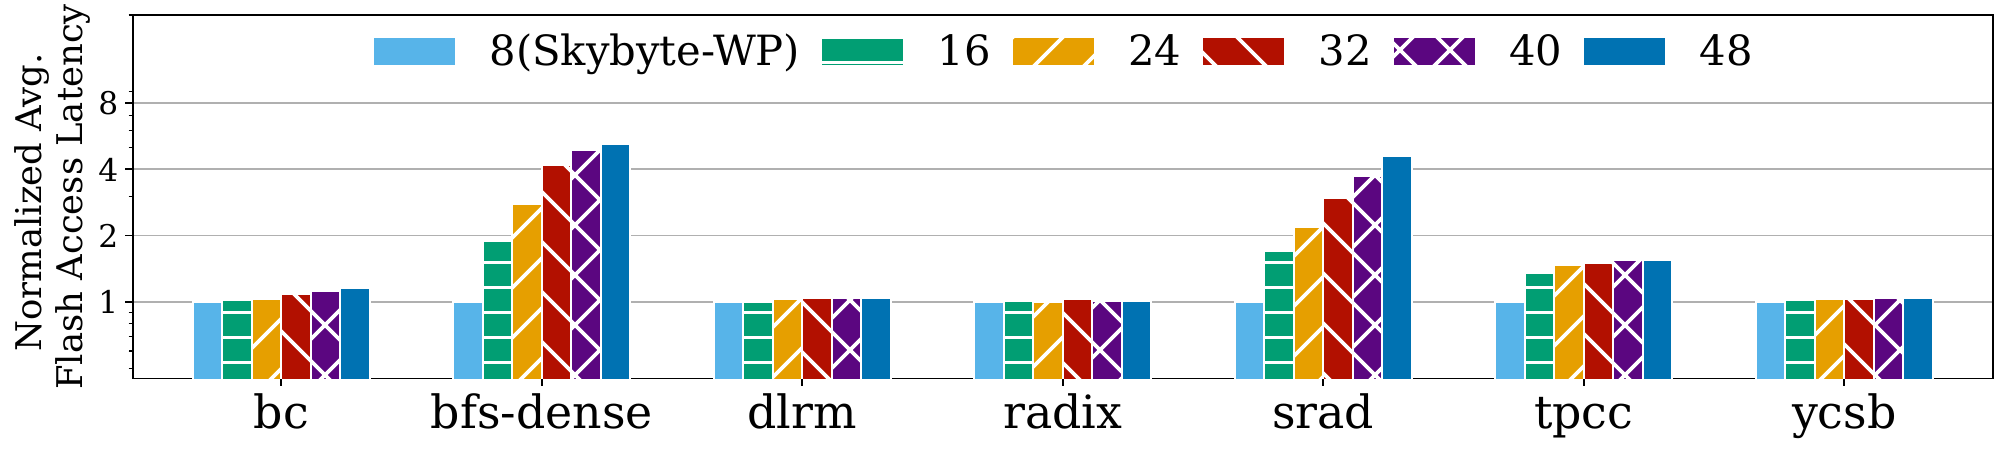}
%    \vspace{-1ex}
%     \caption{\hlB{Average flash read latency of \mbox{\pname{}-Full} as we increase the number of threads (normalized to \mbox{\pname{}-WP} with 8 threads).}}
%     \label{fig:eval_ltcy_vary_threads}
%       \vspace{-1ex}
% \end{figure}

% \hlB{We study the performance impact of varying the number of application threads in Figure \mbox{\ref{fig:eval_ltcy_vary_threads}}.
% As we increase the number of application threads, the number of concurrent SSD accesses increases. As a result, the latency of accessing flash chips may also increase due to queuing delays.
% % The potential of this latency degradation is closely correlated with the flash access pattern of the workload.
% For workloads (e.g., \mbox{\texttt{bfs-dense} and \texttt{srad}}) that have higher flash read latency under \mbox{\pname{-WP}} (see Table \mbox{\ref{tab:wp_read-latency}}), they experience worse latency degradation with more threads (up to 5$\times$ with 48 threads).
% However, the end-to-end application performance is still better with more threads, because the SSD bandwidth utilization is higher (see Figure \mbox{\ref{fig:eval_thpt_vary_threads}}), and the longer latency can still be effectively hidden by the coordinated context switch mechanism.}
